# Supplementary material for: Reducing Unintended Bias of ML Models on Tabular and Textual Data
Source: arXiv:2108.02662 source file (2021-08-05)
Supplement: Supplementary file 1 [file findk_unfair_counter.tex]

% Please add the following required packages to your document preamble:
% \usepackage{multirow}
\begin{table}[]
\centering
\setlength{\tabcolsep}{3pt}
\caption{Number of times that LR classifiers are deemed unfair: Effects of the variation of $\alpha$ on the process fairness assessment.}
\label{tb:unfair_counter_LR}
\begin{tabular}{|r|r|r|llllll|}
\hline
                      & \multirow{2}{*}{\textbf{Dataset}}            & \multirow{2}{*}{\textbf{Selection}} & \multicolumn{6}{c|}{$\alpha$}     \\
                      &                  &  & 0.5   & 1     & 1.5   & 2     & 2.5   & 3     \\
\hline
\multirow{12}{*}{\rotcell[c]{LR}} & \multirow{4}{*}{German} & \textit{LIME+RS}   & \textbf{47}  & 42 & 31  & 23 & 13  & 8  \\
                     &                         & \textit{LIME+SP}   & \textbf{50}  & \textbf{49} & 43  & 39 & 29  & 24 \\
                     &                         & \textit{SHAP+RS}   & \textbf{50}  & \textbf{50} & \textbf{50}  & \textbf{47} & \textbf{45}  & 43 \\
                     &                         & \textit{SHAP+SP}   & \textbf{50}  & \textbf{50} & \textbf{50}  & \textbf{49} & \textbf{45}  & 43 \\
\cline{2-9}
                     & \multirow{4}{*}{Adult}  & \textit{LIME+RS}   & \textbf{46}   &  \textbf{46}  &  \textbf{46}   &  \textbf{46}    &  44   &  44  \\
                     &                         & \textit{LIME+SP}   & \textbf{49} & \textbf{49} & \textbf{49} & \textbf{49} & \textbf{49} & \textbf{49}   \\
                     &                         & \textit{SHAP+RS}   & \textbf{48} & \textbf{48} & \textbf{48} & \textbf{48} & \textbf{48} & \textbf{45}    \\
                     &                         & \textit{SHAP+SP}   & \textbf{50} & \textbf{50} & \textbf{50} & \textbf{50} & \textbf{49} & \textbf{49}   \\
\cline{2-9}
                     & \multirow{4}{*}{LSAC}   & \textit{LIME+RS}   & \textbf{47}  & 28 & 10  & 6  & 1   & 0  \\
                     &                         & \textit{LIME+SP}   & 35  & 22 & 14  & 4  & 0   & 0  \\
                     &                         & \textit{SHAP+RS}   & \textbf{48}  & 42 & 30  & 22 & 18  & 12 \\
                     &                         & \textit{SHAP+SP}   & \textbf{50}  & \textbf{45} & 36  & 26 & 19  & 14 \\
\hline
\end{tabular}
\end{table}

% Please add the following required packages to your document preamble:
% \usepackage{multirow}
\begin{table}[]
\centering
\setlength{\tabcolsep}{3pt}
\caption{Number of times that BAG classifiers are deemed unfair: Effects of the variation of $\alpha$ on the process fairness assessment.}
\label{tb:unfair_counter_BAG}
\begin{tabular}{|r|r|r|llllll|}
\hline
                      & \multirow{2}{*}{\textbf{Dataset}}            & \multirow{2}{*}{\textbf{Selection}} & \multicolumn{6}{c|}{$\alpha$}     \\
                      &                  &  & 0.5   & 1     & 1.5   & 2     & 2.5   & 3     \\
\hline
\multirow{12}{*}{\rotcell[c]{BAG}} & \multirow{4}{*}{German} & \textit{LIME+RS}   & 33  & 31 & 24  & 18 & 8   & 2  \\
                      &                         & \textit{LIME+SP}   & 41  & 41 & 41  & 40 & 30  & 21 \\
                      &                         & \textit{SHAP+RS}   & 37  & 37 & 33  & 26 & 22  & 19 \\
                      &                         & \textit{SHAP+SP}   & \textbf{45}  & \textbf{45} & 43  & 36 & 31  & 26 \\
\cline{2-9}
                      & \multirow{4}{*}{Adult}  & \textit{LIME+RS}   & \textbf{49} & \textbf{49} & \textbf{49} & \textbf{49} & \textbf{45} & 40   \\
                      &                         & \textit{LIME+SP}   & \textbf{50} & \textbf{50} & \textbf{50} & \textbf{50} & \textbf{50} & \textbf{50}   \\
                      &                         & \textit{SHAP+RS}   & \textbf{49} & \textbf{49} & \textbf{49} & \textbf{49} & \textbf{45} & 40   \\
                      &                         & \textit{SHAP+SP}   & \textbf{50} & \textbf{50} & \textbf{50} & 39 & 11 & 2   \\
\cline{2-9}
                      & \multirow{4}{*}{LSAC}   & \textit{LIME+RS}   & \textbf{50}  & \textbf{49} & 43  & 32 & 24  & 21 \\
                      &                         & \textit{LIME+SP}   & \textbf{50}  & \textbf{50} & \textbf{50}  & \textbf{50} & \textbf{49}  & 44 \\
                      &                         & \textit{SHAP+RS}   & \textbf{50}  & 32 & 24  & 17 & 14  & 11 \\
                      &                         & \textit{SHAP+SP}   & \textbf{49}  & 44 & 33  & 26 & 14  & 11 \\
\hline
\end{tabular}
\end{table}

% Please add the following required packages to your document preamble:
% \usepackage{multirow}
\begin{table}[]
\centering
\setlength{\tabcolsep}{3pt}
\caption{Number of times that RF classifiers are deemed unfair: Effects of the variation of $\alpha$ on the process fairness assessment.}
\label{tb:unfair_counter_RF}
\begin{tabular}{|r|r|r|llllll|}
\hline
                      & \multirow{2}{*}{\textbf{Dataset}}            & \multirow{2}{*}{\textbf{Selection}} & \multicolumn{6}{c|}{$\alpha$}     \\
                      &                  &  & 0.5   & 1     & 1.5   & 2     & 2.5   & 3     \\
\hline
\multirow{12}{*}{\rotcell[c]{RF}} & \multirow{4}{*}{German} & \textit{LIME+RS}   & \textbf{49}  & 43 & 25  & 8  & 2   & 1  \\
                     &                         & \textit{LIME+SP}   & \textbf{50}  & \textbf{50} & \textbf{50}  & \textbf{50} & \textbf{47}  & \textbf{46} \\
                     &                         & \textit{SHAP+RS}   & \textbf{50}  & \textbf{48} & 39  & 29 & 23  & 18 \\
                     &                         & \textit{SHAP+SP}   & \textbf{50}  & \textbf{47} & 33  & 27 & 22  & 17 \\
\cline{2-9}
                     & \multirow{4}{*}{Adult}  & \textit{LIME+RS}   &  \textbf{50}  & \textbf{50} & \textbf{48}  & 38 & 18  & 6 \\
                     &                         & \textit{LIME+SP}   &  \textbf{50}  & \textbf{50} & \textbf{50}  & \textbf{48} & 40  & 27 \\
                     &                         & \textit{SHAP+RS}   &  \textbf{50}  & \textbf{50} & \textbf{50}  & \textbf{50} & \textbf{46}  & 41 \\
                     &                         & \textit{SHAP+SP}   &  \textbf{50}  & \textbf{50} & \textbf{50}  & \textbf{48} & \textbf{47}  & 38 \\
\cline{2-9}
                     & \multirow{4}{*}{LSAC}   & \textit{LIME+RS}   & \textbf{49}  & 38 & 16  & 10 & 6   & 6  \\
                     &                         & \textit{LIME+SP}   & \textbf{50}  & \textbf{49} & \textbf{48}  & \textbf{48} & \textbf{48}  & \textbf{48} \\
                     &                         & \textit{SHAP+RS}   & \textbf{47}  & 40 & 21  & 13 & 7   & 3  \\
                     &                         & \textit{SHAP+SP}   & \textbf{49}  & 37 & 23  & 13 & 8   & 4 \\
\hline
\end{tabular}
\end{table}

% Please add the following required packages to your document preamble:
% \usepackage{multirow}
\begin{table}[]
\centering
\setlength{\tabcolsep}{3pt}
\caption{Number of times that ADA classifiers are deemed unfair: Effects of the variation of $\alpha$ on the process fairness assessment.}
\label{tb:unfair_counter_ADA}
\begin{tabular}{|r|r|r|llllll|}
\hline
                      & \multirow{2}{*}{\textbf{Dataset}}            & \multirow{2}{*}{\textbf{Selection}} & \multicolumn{6}{c|}{$\alpha$}     \\
                      &                  &  & 0.5   & 1     & 1.5   & 2     & 2.5   & 3     \\
\hline
\multirow{12}{*}{\rotcell[c]{ADA}} & \multirow{4}{*}{German} & \textit{LIME+RS}   & \textbf{48}  & \textbf{48} & \textbf{48}  & \textbf{46} & \textbf{45}  & 44 \\
                      &                         & \textit{LIME+SP}   & \textbf{50}  & \textbf{50} & \textbf{50}  & \textbf{50} & \textbf{50}  & \textbf{50} \\
                      &                         & \textit{SHAP+RS}   & \textbf{48}  & 43 & 31  & 23 & 15  & 13 \\
                      &                         & \textit{SHAP+SP}   & \textbf{47}  & 42 & 34  & 30 & 24  & 20 \\
\cline{2-9}
                      & \multirow{4}{*}{Adult}  & \textit{LIME+RS}   & \textbf{50}  & \textbf{50} & \textbf{49}  & \textbf{35} & 13  & 2 \\
                      &                         & \textit{LIME+SP}   & \textbf{50}  & \textbf{50} & \textbf{49}  & 43 & 19  & 4 \\
                      &                         & \textit{SHAP+RS}   & \textbf{50}  & \textbf{50} & \textbf{49}  & \textbf{48} & \textbf{47}  & \textbf{47} \\
                      &                         & \textit{SHAP+SP}   & \textbf{50}  & \textbf{49} & \textbf{49}  & \textbf{49} & \textbf{47}  & \textbf{47} \\
\cline{2-9}
                      & \multirow{4}{*}{LSAC}   & \textit{LIME+RS}   & 44  & 32 & 20  & 11 & 5   & 4  \\
                      &                         & \textit{LIME+SP}   & \textbf{46}  & 34 & 22  & 11 & 9   & 4  \\
                      &                         & \textit{SHAP+RS}   & \textbf{50}  & 42 & 30  & 21 & 8   & 6  \\
                      &                         & \textit{SHAP+SP}   & \textbf{50}  & \textbf{47} & 39  & 26 & 12  & 7 \\
\hline
\end{tabular}
\end{table}
