# Supplementary material for: Reducing Unintended Bias of ML Models on Tabular and Textual Data
Source: arXiv:2108.02662 source file (2021-08-05)
Supplement: Supplementary file 2 [file old_tables.tex]

\begin{table}[]
\centering
\setlength{\tabcolsep}{1pt}
\caption{Average value of $k$ for LR classifiers: Effects of the variation of $\alpha$ over the number of features kept by \FK.}
\label{tb:k_LR}
\begin{tabular}{|r|r|r|rlrlrlrlrlrl|}
\hline
                      & \multirow{2}{*}{\textbf{Dataset}}            & \multirow{2}{*}{\textbf{Selection}} & \multicolumn{12}{c|}{$\alpha$}     \\
                      &                  &  & \multicolumn{2}{c}{0.5}   & \multicolumn{2}{c}{1}     & \multicolumn{2}{c}{1.5}   & \multicolumn{2}{c}{2}     & \multicolumn{2}{c}{2.5}   & \multicolumn{2}{c|}{3}    \\
\hline
\multirow{12}{*}{\rotcell[c]{LR}} & \multirow{4}{*}{German} & \textit{LIME+RS} & \textbf{9.9} & (\textbf{47}) & \textbf{8.7} & (42) & \textbf{6.8} & (31) & 5.5 & (23) & 3.5 & (13) & 2.6 & (8) \\
                     &                         & \textit{LIME+SP}   & \textbf{9.7} & (\textbf{50})  & \textbf{8.2} & (\textbf{49})  & \textbf{6.1} & (43)  & \textbf{4.5} & (39)  & 2.1 & (29)  & 1.3 & (24)  \\
                     &                         & \textit{SHAP+RS}   & \textbf{10.0} & (\textbf{50}) & \textbf{9.9} & (\textbf{50})  & \textbf{9.5} & (\textbf{50})  & \textbf{7.4} & (\textbf{47})  & \textbf{5.7} & (\textbf{45})  & \textbf{3.8} & (43)  \\
                     &                         & \textit{SHAP+SP}   & \textbf{10.0}  & (\textbf{50}) & \textbf{9.8}  & (\textbf{50}) & \textbf{8.9}  & (\textbf{50}) & \textbf{7.0}  & (\textbf{49}) & \textbf{5.4}  & (\textbf{45}) & \textbf{4.0}  & (43) \\
\cline{2-14}
                     & \multirow{4}{*}{Adult}  & \textit{LIME+RS}   & \textbf{10.0} & (\textbf{46}) & \textbf{10.0} & (\textbf{46}) & \textbf{10.0} & (\textbf{46}) & \textbf{9.9} & (\textbf{46}) & \textbf{9.9}  & (44) & \textbf{9.8}  & (44) \\
                     &                         & \textit{LIME+SP}   & \textbf{10.0} & (\textbf{49}) & \textbf{10.0} & (\textbf{49}) & \textbf{10.0} & (\textbf{49}) & \textbf{10.0} & (\textbf{49})  & \textbf{9.9} & (\textbf{49}) & \textbf{9.8} & (\textbf{49}) \\
                     &                         & \textit{SHAP+RS}   & \textbf{10.0} & (\textbf{48}) & \textbf{10.0} & (\textbf{48})  & \textbf{10.0} & (\textbf{48})  & \textbf{10.0} & (\textbf{48})  & \textbf{9.8} & (\textbf{48})  & \textbf{9.7} & (\textbf{45})  \\
                     &                         & \textit{SHAP+SP}   & \textbf{10.0} & (\textbf{50}) & \textbf{9.9} & (\textbf{50}) & \textbf{9.8} & (\textbf{50}) & \textbf{9.7} & (\textbf{50}) & \textbf{9.6} & (\textbf{49}) & \textbf{9.3} & (\textbf{49}) \\
\cline{2-14}
                     & \multirow{4}{*}{LSAC}   & \textit{LIME+RS}   & \textbf{8.6} & (\textbf{47})  & 6.4 & (28)  & 4.0 & (10)  & 2.5 & (6)  & 1.8 & (1)  & 1.3 & (0)  \\
                     &                         & \textit{LIME+SP}   & 7.7 & (35) & 5.1 & (22) & 3.1 & (14) & 1.7 & (4) & 1.1 & (0) & 1.0 & (0) \\
                     &                         & \textit{SHAP+RS}   & \textbf{8.5} & (\textbf{48}) & \textbf{6.6} & (42) & 4.5 & (30) & 3.2 & (22) & 2.5 & (18) & 2.0 & (12) \\
                     &                         & \textit{SHAP+SP}   & \textbf{8.3} & (\textbf{50}) & \textbf{6.1} & (\textbf{45}) & \textbf{4.4} & (36) & 3.2 & (26) & 2.3 & (19) & 1.7 & (14)\\
\hline
\end{tabular}
\end{table}

%%%%%%%%%%%%%%%%%%%%%%%%%%%%%%%%%%%%%
\begin{table}[]
\centering
\setlength{\tabcolsep}{1pt}
\caption{Average value of $k$ for BAG classifiers: Effects of the variation of $\alpha$ over the number of features kept by \FK.}
\label{tb:k_BAG}
\begin{tabular}{|r|r|r|rlrlrlrlrlrl|}
\hline
                      & \multirow{2}{*}{\textbf{Dataset}}            & \multirow{2}{*}{\textbf{Selection}} & \multicolumn{12}{c|}{$\alpha$}     \\
                      &                  &  & \multicolumn{2}{c}{0.5}   & \multicolumn{2}{c}{1}     & \multicolumn{2}{c}{1.5}   & \multicolumn{2}{c}{2}     & \multicolumn{2}{c}{2.5}   & \multicolumn{2}{c|}{3}    \\
\hline
%\multirow{12}{*}{\rotcell[c]{BAG}} & \multirow{4}{*}{German} & \textit{LIME+RS}   & 10.00 & 9.58  & 8.18 & 6.38 & 4.26 & 2.82 \\
%                      &                         & \textit{LIME+SP}   & \textbf{10.00} & \textbf{10.00} & \textbf{9.74} & 9.08 & 7.04 & 4.86 \\
%                      &                         & \textit{SHAP+RS}   & 9.92  & 9.80  & 8.78 & 7.16 & 5.86 & 4.86 \\
%                      &                         & \textit{SHAP+SP}   & \textbf{10.00} & \textbf{9.78}  & \textbf{9.12} & 7.72 & 6.58 & 5.50 \\
%\cline{2-9}
%                      & \multirow{4}{*}{Adult}  & \textit{LIME+RS}   & \textbf{10.0} & \textbf{10.0} & \textbf{10.0} & \textbf{9.58} & \textbf{8.32} & 6.82 \\
%                      &                         & \textit{LIME+SP}   & \textbf{10.0} & \textbf{10.0} & \textbf{10.0} & \textbf{9.64} & \textbf{8.52} & \textbf{7.32} \\
%                      &                         & \textit{SHAP+RS}   & \textbf{10.0} & \textbf{10.0} & \textbf{10.0} & \textbf{9.62} & \textbf{8.30} & 7.08 \\
%                      &                         & \textit{SHAP+SP}   & \textbf{10.0} & \textbf{10.0} & \textbf{8.84} & 5.84 & 2.32 & 1.32 \\
%\cline{2-9}
%                      & \multirow{4}{*}{LSAC}   & \textit{LIME+RS}   & \textbf{7.74}  & \textbf{5.64}  & \textbf{4.04} & \textbf{2.68} & 1.98 & 1.56 \\
%                      &                         & \textit{LIME+SP}   & \textbf{9.72}  & \textbf{8.76}  & \textbf{7.86} & \textbf{7.00} & \textbf{5.96} & \textbf{4.84} \\
%                      &                         & \textit{SHAP+RS}   & \textbf{8.34}  & \textbf{5.98}  & 4.46 & 3.04 & 2.56 & 2.08 \\
%                      &                         & \textit{SHAP+SP}   & \textbf{8.70}  & \textbf{6.88}  & \textbf{5.10} & 3.76 & 2.82 & 2.22 \\
%\hline

\multirow{12}{*}{\rotcell[c]{BAG}} & \multirow{4}{*}{German} & \textit{LIME+RS}   & 10.0 & (33) & 9.58 & (31) & 8.18 & (24) & 6.38 & (18) & 4.26 & (8) & 2.82 & (2) \\
                      &                         & \textit{LIME+SP}   & \textbf{10.0} & (41) & \textbf{10.0} & (41) & \textbf{9.74} & (41) & 9.08 & (40) & 7.04 & (30) & 4.86 & (21) \\
                      &                         & \textit{SHAP+RS}   & 9.92 & (37) & 9.80 & (37) & 8.78 & (33) & 7.16 & (26) & 5.86 & (22) & 4.86 & (19) \\
                      &                         & \textit{SHAP+SP}   & \textbf{10.0} & (\textbf{45}) & \textbf{9.78} & (\textbf{45}) & \textbf{9.12} & (43) & 7.72 & (36) & 6.58 & (31) & 5.50 & (26) \\
\cline{2-9}
                      & \multirow{4}{*}{Adult}  & \textit{LIME+RS}   & \textbf{10.0} & (\textbf{49}) & \textbf{10.0} & (\textbf{49}) & \textbf{10.0} & (\textbf{49}) & \textbf{9.58} & (\textbf{49}) & \textbf{8.32} & (\textbf{45}) & 6.82 & (40) \\
                      &                         & \textit{LIME+SP}   & \textbf{10.0} & (50) & \textbf{10.0} & (50) & \textbf{10.0} & (50) & \textbf{9.64} & (50) & \textbf{8.52} & (50) & \textbf{7.32} & (50) \\
                      &                         & \textit{SHAP+RS}   & \textbf{10.0} & (\textbf{49}) & \textbf{10.0} & (\textbf{49}) & \textbf{10.0} & (\textbf{49}) & \textbf{9.62} & (\textbf{49}) & \textbf{8.30} & (\textbf{45}) & 7.08 & (40) \\
                      &                         & \textit{SHAP+SP}   & \textbf{10.0} & (\textbf{50}) & \textbf{10.0} & (\textbf{50}) & \textbf{8.84} & (\textbf{50}) & 5.84 & (39) & 2.32 & (11) & 1.32 & (2) \\
\cline{2-9}
                      & \multirow{4}{*}{LSAC}   & \textit{LIME+RS}   & \textbf{7.74} & (\textbf{50})  & \textbf{5.64} & (\textbf{49}) & \textbf{4.04} & (43) & \textbf{2.68} & (32) & 1.98 & (24) & 1.56 & (21) \\
                      &                         & \textit{LIME+SP}   & \textbf{9.72} & (\textbf{50})  & \textbf{8.76} & (\textbf{50}) & \textbf{7.86} & (\textbf{50}) & \textbf{7.00} & (\textbf{50}) & \textbf{5.96} & (\textbf{49}) & \textbf{4.84} & (44) \\
                      &                         & \textit{SHAP+RS}   & \textbf{8.34} & (\textbf{50}) & \textbf{5.98} & (32) & 4.46 & (24) & 3.04 & (17) & 2.56 & (14) & 2.08 & (11) \\
                      &                         & \textit{SHAP+SP}   & \textbf{8.70} & (\textbf{49})  & \textbf{6.88}  & (44) & \textbf{5.10} & (33) & 3.76 & (26) & 2.82 & (14) & 2.22 & (11)\\
\hline
\end{tabular}
\end{table}

%%%%%%%%%%%%%%%%%%%%%%%%%%%%%%%%%%%%%%
%\begin{table}[]
%\centering
%\setlength{\tabcolsep}{3pt}
%\caption{Average value of $k$ for RF classifiers: Effects of the variation of $\alpha$ over the number of features kept by \FK.}
%\label{tb:k_RF}
%\begin{tabular}{|r|r|r|rlrlrlrlrlrl|}
%\hline
%                      & \multirow{2}{*}{\textbf{Dataset}}            & \multirow{2}{*}{\textbf{Selection}} & \multicolumn{12}{c|}{$\alpha$}     \\
%                      &                  &  & \multicolumn{2}{c}{0.5}   & \multicolumn{2}{c}{1}     & \multicolumn{2}{c}{1.5}   & \multicolumn{2}{c}{2}     & \multicolumn{2}{c}{2.5}   & \multicolumn{2}{c|}{3}    \\
%\hline
%%\multirow{12}{*}{\rotcell[c]{RF}} & \multirow{4}{*}{German} & \textit{LIME+RS}   & \textbf{9.90}  & \textbf{8.30} & 5.18 & 2.72 & 1.54 & 1.18 \\
%%                     &                         & \textit{LIME+SP}   & \textbf{10.00} & \textbf{9.98} & \textbf{9.74} & \textbf{8.54} & \textbf{6.96} & \textbf{5.46} \\
%%                     &                         & \textit{SHAP+RS}   & \textbf{9.92}  & \textbf{8.98} & \textbf{6.46} & 4.52 & 2.74 & 2.04 \\
%%                     &                         & \textit{SHAP+SP}   & \textbf{9.86}  & \textbf{8.70} & 5.64 & 3.68 & 2.28 & 1.42 \\
%%\cline{2-9}
%%                     & \multirow{4}{*}{Adult}  & \textit{LIME+RS}   & \textbf{9.76}  & \textbf{8.38} & \textbf{7.00} & \textbf{5.48} & 4.44 & 3.64 \\
%%                     &                         & \textit{LIME+SP}   & \textbf{9.30}  & \textbf{7.80} & \textbf{6.76} & \textbf{5.80} & 5.00 & 4.32 \\
%%                     &                         & \textit{SHAP+RS}   & \textbf{10.00}  & \textbf{9.96} & \textbf{9.30} & \textbf{8.12} & \textbf{6.48} & \textbf{5.14} \\
%%                     &                         & \textit{SHAP+SP}   & \textbf{10.00}  & \textbf{9.98} & \textbf{9.38} & \textbf{8.02} & \textbf{6.26} & \textbf{4.94} \\
%%\cline{2-9}
%%                     & \multirow{4}{*}{LSAC}   & \textit{LIME+RS}   & \textbf{6.46}  & \textbf{4.04} & 2.02 & 1.46 & 1.10 & 1.02 \\
%%                     &                         & \textit{LIME+SP}   & \textbf{8.92}  & \textbf{7.30} & \textbf{5.38} & \textbf{3.66} & 2.66 & 1.96 \\
%%                     &                         & \textit{SHAP+RS}   & \textbf{7.80}  & \textbf{5.80} & 3.88 & 2.48 & 1.76 & 1.40 \\
%%                     &                         & \textit{SHAP+SP}   & \textbf{8.18}  & \textbf{5.78} & 4.04 & 2.86 & 2.10 & 1.70 \\
%%\hline
%
%\multirow{12}{*}{\rotcell[c]{RF}} & \multirow{4}{*}{German} & \textit{LIME+RS}   & \textbf{9.90} & (\textbf{49}) & \textbf{8.30} & (43) & 5.18 & (25) & 2.72 & (8) & 1.54& (2) & 1.18 & (2) \\
%                     &                         & \textit{LIME+SP}   & \textbf{10.00} & (\textbf{50}) & \textbf{9.98} & (\textbf{50}) & \textbf{9.74} & (\textbf{50}) & \textbf{8.54} & (\textbf{50}) & \textbf{6.96} & (\textbf{47}) & \textbf{5.46} & (\textbf{46}) \\
%                     &                         & \textit{SHAP+RS}   & \textbf{9.92} & (\textbf{50})  & \textbf{8.98} & (\textbf{48}) & \textbf{6.46} & (39) & 4.52 & (29) & 2.74 & (23) & 2.04 & (18) \\
%                     &                         & \textit{SHAP+SP}   & \textbf{9.86} & (\textbf{50}) & \textbf{8.70} & (\textbf{47}) & 5.64 & (33) & 3.68 & (27) & 2.28 & (22) & 1.42 & (17) \\
%\cline{2-14}
%                     & \multirow{4}{*}{Adult}  & \textit{LIME+RS}   & \textbf{9.76} & (\textbf{50}) & \textbf{8.38} & (\textbf{50}) & \textbf{7.00} & (\textbf{48}) & \textbf{5.48} & (38) & 4.44 & (18) & 3.64 & (6) \\
%                     &                         & \textit{LIME+SP}   & \textbf{9.30} & (\textbf{50}) & \textbf{7.80} & (\textbf{50}) & \textbf{6.76} & (\textbf{50}) & \textbf{5.80} & (\textbf{48}) & 5.00 & (40) & 4.32 & (27) \\
%                     &                         & \textit{SHAP+RS}   & \textbf{10.00} & (\textbf{50}) & \textbf{9.96} & (\textbf{50}) & \textbf{9.30} & (\textbf{50}) & \textbf{8.12} & (\textbf{50}) & \textbf{6.48} & (\textbf{46}) & \textbf{5.14} & (41) \\
%                     &                         & \textit{SHAP+SP}   & \textbf{10.00} & (\textbf{50})  & \textbf{9.98} & (\textbf{50})  & \textbf{9.38} & (\textbf{50}) & \textbf{8.02} & (\textbf{48}) & \textbf{6.26} & (\textbf{47}) & \textbf{4.94} & (38) \\
%\cline{2-14}
%                     & \multirow{4}{*}{LSAC}   & \textit{LIME+RS}   & \textbf{6.46} & (\textbf{49}) & \textbf{4.04} & (38) & 2.02& (16) & 1.46 & (10) & 1.10 & (6) & 1.02 & (6)\\
%                     &                         & \textit{LIME+SP}   & \textbf{8.92} & (\textbf{50})  & \textbf{7.30} & (\textbf{49}) & \textbf{5.38} & (\textbf{48}) & \textbf{3.66} & (\textbf{48}) & 2.66 & (\textbf{48}) & 1.96 & (\textbf{48}) \\
%                     &                         & \textit{SHAP+RS}   & \textbf{7.80} & (\textbf{47}) & \textbf{5.80} & (40) & 3.88 & (21) & 2.48 & (13) & 1.76 & (7) & 1.40 (3) \\
%                     &                         & \textit{SHAP+SP}   & \textbf{8.18} & (\textbf{49}) & \textbf{5.78} & (37) & 4.04 & (23) & 2.86 & (13) & 2.10 & (8) & 1.70 & (4) \\
%\hline
%\end{tabular}
%\end{table}

%%%%%%%%%%%%%%%%%%%%%%%%%%%%%%%%%%%%%% 
%\begin{table}[]
%\centering
%\setlength{\tabcolsep}{3pt}
%\caption{Average value of $k$ for ADA classifiers: Effects of the variation of $\alpha$ over the number of features kept by \FK.}
%\label{tb:k_ADA}
%\begin{tabular}{|r|r|r|rlrlrlrlrlrl|}
%\hline
%                      & \multirow{2}{*}{\textbf{Dataset}}            & \multirow{2}{*}{\textbf{Selection}} & \multicolumn{12}{c|}{$\alpha$}     \\
%                      &                  &  & \multicolumn{2}{c}{0.5}   & \multicolumn{2}{c}{1}     & \multicolumn{2}{c}{1.5}   & \multicolumn{2}{c}{2}     & \multicolumn{2}{c}{2.5}   & \multicolumn{2}{c|}{3}    \\
%\hline
%%\multirow{12}{*}{\rotcell[c]{ADA}} & \multirow{4}{*}{German} & \textit{LIME+RS}   & \textbf{10}    & \textbf{10}    & \textbf{9.76}  & \textbf{9.4}   & \textbf{9.2}   & \textbf{9.04}  \\
%%                      &                         & \textit{LIME+SP}   & \textbf{10.00} & \textbf{10.00} & \textbf{10.00} & \textbf{10.00} & \textbf{10.00} & \textbf{10.00} \\
%%                      &                         & \textit{SHAP+RS}   & \textbf{10.00} & \textbf{8.78}  & 6.44  & 4.28  & 3.24  & 2.90  \\
%%                      &                         & \textit{SHAP+SP}   & \textbf{9.98}  & \textbf{8.68}  & 6.78  & 5.82  & 4.92  & 4.04  \\
%%\cline{2-9}
%%                      & \multirow{4}{*}{Adult}  & \textit{LIME+RS}   & \textbf{10.00} & \textbf{10.00} & \textbf{8.22} & \textbf{5.54} & {3.40} & {2.20} \\
%%                      &                         & \textit{LIME+SP}   & \textbf{10.00} & \textbf{9.90} & \textbf{7.98} & \textbf{5.74} & {3.84} & {2.48} \\
%%                      &                         & \textit{SHAP+RS}   & \textbf{10.00} & \textbf{9.02} & \textbf{6.62} & \textbf{4.76} & {3.28} & {2.38} \\
%%                      &                         & \textit{SHAP+SP}   & \textbf{10.00} & \textbf{9.16} & \textbf{7.22} & \textbf{5.36} & \textbf{4.06} & \textbf{2.82} \\
%%\cline{2-9}
%%                      & \multirow{4}{*}{LSAC}   & \textit{LIME+RS}   & \textbf{6.98}  & \textbf{4.52}  & 3.02  & 1.92  & 1.28  & 1.12  \\
%%                      &                         & \textit{LIME+SP}   & \textbf{7.08}  & \textbf{5.06}  & 3.44  & 2.22  & 1.78  & 1.28  \\
%%                      &                         & \textit{SHAP+RS}   & \textbf{8.68}  & \textbf{6.52}  & 4.78  & 3.34  & 2.08  & 1.52  \\
%%                      &                         & \textit{SHAP+SP}   & \textbf{8.84}  & \textbf{7.08}  & \textbf{5.42}  & 3.84  & 2.68  & 1.90 \\
%%\hline
%
%
%\multirow{12}{*}{\rotcell[c]{ADA}} & \multirow{4}{*}{German} & \textit{LIME+RS}   & \textbf{10}    & \textbf{10}    & \textbf{9.76}  & \textbf{9.4}   & \textbf{9.2}   & \textbf{9.04}  \\
%                      &                         & \textit{LIME+SP}   & \textbf{10.00} & (\textbf{50}) & \textbf{10.00} & (\textbf{50}) & \textbf{10.00} & (\textbf{50}) & \textbf{10.00} & (\textbf{50}) & \textbf{10.00} & (\textbf{50}) & \textbf{10.00} & (\textbf{50}) \\
%                      &                         & \textit{SHAP+RS}   & \textbf{10.00} & (\textbf{48}) & \textbf{8.78} & (43) & 6.44 & (31) & 4.28 & (23) & 3.24 & (15) & 2.90 & (13) \\
%                      &                         & \textit{SHAP+SP}   & \textbf{9.98} & (\textbf{47}) & \textbf{8.68} & (42) & 6.78 & (34) & 5.82 & (30) & 4.92 & (24) & 4.04 & (20) \\
%\cline{2-14}
%                      & \multirow{4}{*}{Adult}  & \textit{LIME+RS}   & \textbf{10.00} & (\textbf{50}) & \textbf{10.00} & (\textbf{50}) & \textbf{8.22} & (\textbf{49}) & \textbf{5.54} & (35) & {3.40} & (13) & {2.20} & (2)\\
%                      &                         & \textit{LIME+SP}   & \textbf{10.00} & (\textbf{50}) & \textbf{9.90} & (\textbf{50}) & \textbf{7.98} & (\textbf{49}) & \textbf{5.74} & (43) & {3.84} & (19) & {2.48} & (4) \\
%                      &                         & \textit{SHAP+RS}   & \textbf{10.00} & (\textbf{50}) & \textbf{9.02} & (\textbf{50}) & \textbf{6.62} & (\textbf{49}) & \textbf{4.76} & (\textbf{48}) & {3.28} & (\textbf{47}) & {2.38} & (\textbf{47})\\
%                      &                         & \textit{SHAP+SP}   & \textbf{10.00} & (\textbf{50}) & \textbf{9.16} & (\textbf{49}) & \textbf{7.22} & (\textbf{49}) & \textbf{5.36} & (\textbf{49}) & \textbf{4.06} & (\textbf{47}) & \textbf{2.82} & (\textbf{47})\\
%\cline{2-14}
%                      & \multirow{4}{*}{LSAC}   & \textit{LIME+RS}   & \textbf{6.98} & (44) & \textbf{4.52} & (32) & 3.02 & (20) & 1.92 & (11) & 1.28 & (5) & 1.12 & (4) \\
%                      &                         & \textit{LIME+SP}   & \textbf{7.08} & (\textbf{46}) & \textbf{5.06} & (34) & 3.44 & (22) & 2.22 & (11) & 1.78 & (9) & 1.28 & (4)  \\
%                      &                         & \textit{SHAP+RS}   & \textbf{8.68} & (\textbf{50}) & \textbf{6.52} & (42) & 4.78 & (30) & 3.34 & (21) & 2.08 & (8) & 1.52 & (6) \\
%                      &                         & \textit{SHAP+SP}   & \textbf{8.84} & (\textbf{50}) & \textbf{7.08} & (\textbf{47}) & \textbf{5.42} & (39) & 3.84 & (26) & 2.68 & (12) & 1.90 & (7) \\
%\hline

%\end{tabular}
%\end{table}

%%%%%%%%%%%%%%%%%%%%%%%%%%%%%%%%%%%%%%%%%%%%%
%~~~~~~~~~~~~~~~~~~~~~~~~~~~~~~~~~~~~~~~~~~~~
%%%%%%%%%%%%%%%%%%%%%%%%%%%%%%%%%%%%%%%%%%%%%
